# Supplementary material for: Sim-CLIP: Unsupervised Siamese Adversarial Fine-Tuning for Robust and Semantically-Rich Vision-Language Models
Source: arXiv:2407.14971 source file (2026-04-07)
Supplement: Supplementary file 1 [file Appendix1.tex]

\clearpage

% \begin{enumerate}
% \itemindent=5pt
% \item Appendix \ref{app:suptraining}\hspace{0mm} --- \hspace{0mm} Omitted Proof
%    \item Appendix~\ref{app:exp-detail} \hspace{0mm} --- \hspace{0mm} Experimental Details and Ablations
%    \item Appendix~\ref{app:other-exp} \hspace{0mm} --- \hspace{0mm} Additional Experiments
%      \end{enumerate}

\appendix

\label{app:targeted}

\subsection{Training Hyperparameters ablation.}

In this segment, we delve into the specifics of our experimental setup, exploring different hyperparameter configurations for our Sim-CLIP approach.  All experiments detailed in this paper utilize ViT-L/14 CLIP encoder. Due to the significant computational resources required for training such CLIP model, we leverage an early stopping strategy at 500 adversarial training steps. This strategy allows us to effectively evaluate and compare the performance of Sim-CLIP across different hyperparameter configurations. Initially, we investigate the impact of different optimizers in Sim-CLIP, followed by further experiments adjusting the Learning Rate (LR) and Weight Decay (WD) to identify the optimal configuration for the chosen optimizer. In line with the SOTA adversarial fine-tuning methods (e.g., TeCoA and FARE), we constrain the LR and WD search of our method within the values of 1e-3 to 1e-6 and 1e-3 to 1e-5, respectively.

% In line with the supervised fine-tuning methodology proposed by \cite{mao2022understanding}, we constrain the LR and WD search of our method within the values of 1e-3 to 1e-6 and 1e-3 to 1e-5, respectively.

Next, in Figure \ref{fig:hyperparameterablation}, we illustrate the performance of Sim-CLIP with different hyperparameter configurations. Figure \ref{fig:hyperparameterablation}(a) illustrates our ablation study comparing Sim-CLIP's performance using both SGD and AdamW optimizers. For both optimizers, we maintain LR at 1e-6 and WD at 1e-3. Notably, we observe that Sim-CLIP is highly sensitive to optimizer selection, showing significantly better performance with the AdamW optimizer compared to SGD. Hence, we select AdamW as our final optimizer for Sim-CLIP. Subsequently, we experiment with different LR and WD combinations with AdamW optimizer and present our findings in Figure \ref{fig:hyperparameterablation}(b) and Figure \ref{fig:hyperparameterablation}(c). 
Initially, we explore the combination with the highest LR (1e-3) and the lowest WD (1e-5) within our predefined hyperparameter search bounds. We observe that Sim-CLIP struggles to converge with a higher learning rate, whereas, lowering the learning rates leads to notably better performance. However, when the LR is reduced to lowest value (1e-6) within our search bounds, Sim-CLIP again encounters challenges in achieving convergence. Building on these observations, we find that an LR of 1e-5 coupled with a WD of 1e-4 yields superior results compared to alternative configurations. Additionally, our analysis reveals that Sim-CLIP exhibits some sensitivity to Weight Decay (WD), although not to the extent observed with LR. 

We observe consistent
performance trends with the aforementioned hyperparameter configuration when evaluating the robust accuracy on
the ImageNet dataset, as illustrated in Figure \ref{fig:hyperparameterablation}(c). Unlike traditional accuracy (clean accuracy), which measures performance only considering clean data, robust accuracy provides a more comprehensive assessment using adversarially perturbed samples.
Within the initial 500 training steps, Sim-CLIP demonstrates higher robust accuracy when configured with an LR of 1e-5 and a WD of 1e-4. This finding suggests that the combination of a lower learning rate and a slightly higher weight decay contributes to the enhanced robustness of Sim-CLIP during the early stages of training.
Based on these observations, we determine the optimal Sim-CLIP hyperparameters to be an LR of 1e-5 and a WD of 1e-4.

\begin{figure*}[htb!]
% \setlength{\belowcaptionskip}{-1pt}
% \vspace{-0.1cm}
\centering
%\footnotesize
\begin{tabular}{ccc}
\includegraphics[width=0.32\linewidth]{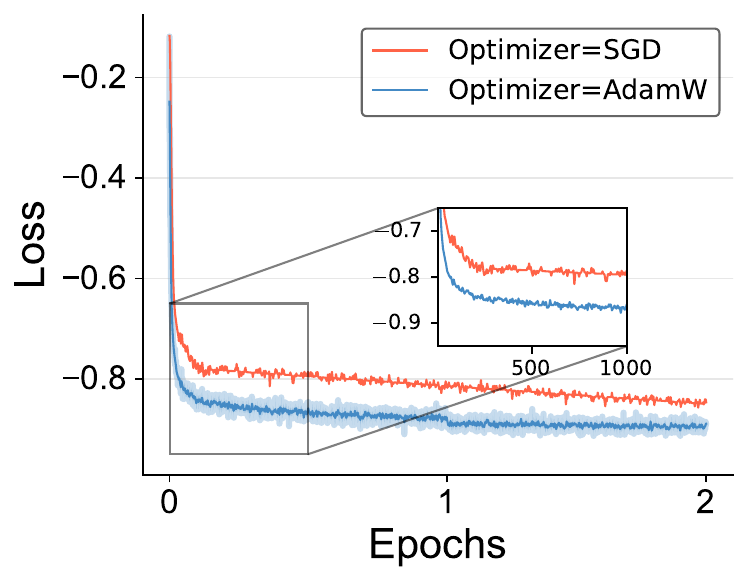}
&
\includegraphics[width=0.32\linewidth]{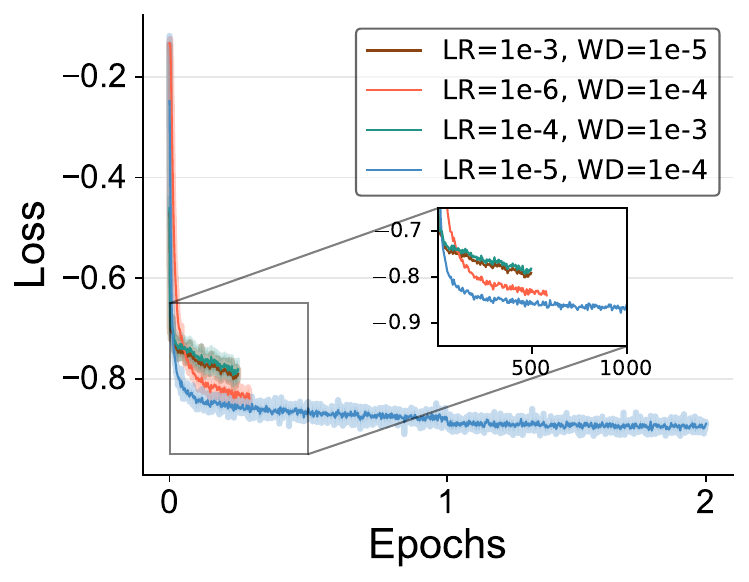}
&
\includegraphics[width=0.32\linewidth]{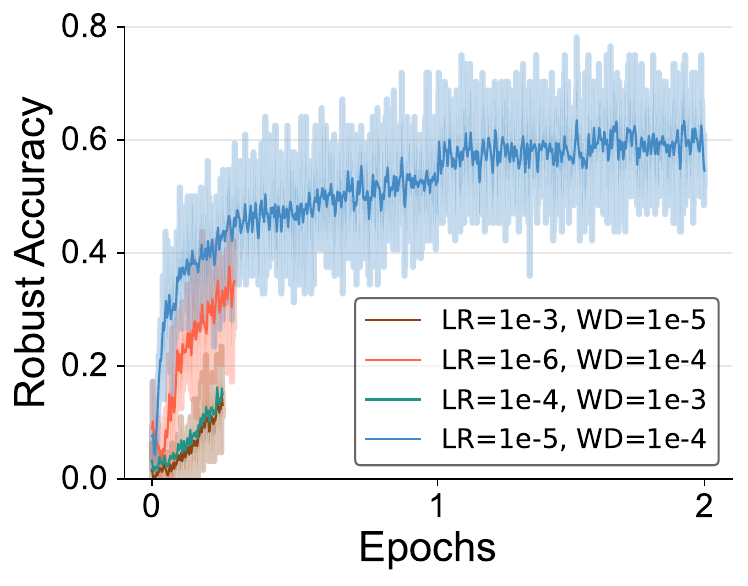}
\\\vspace{-0.1mm}
 (a) & (b) & (c) 
\end{tabular}

\caption{\textbf{Training hyperparameter ablation for Sim-CLIP.}  \textbf{Left plot}: comparing loss minimization performance between the SGD and AdamW optimizers. Sim-CLIP generalizes better with AdamW optimizer. \textbf{Middle plot:} comparison of adversarial training loss minimization with AdamW optimizer across different Learning Rates (LR) and Weight-decay (WD). \textbf{Right plot:} robust accuracy comparison on different LR and WD with AdamW optimizer.  }
\label{fig:hyperparameterablation}
\end{figure*}
